# Supplementary material for: O2A: One-shot Observational learning with Action vectors
Source: arXiv:1810.07483 source file (2020-12-21)
Supplement: Supplementary file 1 [file appendix.tex]

hi
